# Supplementary material for: Strategies for Asymptotic Normalization
Source: arXiv:2204.08772 source file (2022-05-23)
Supplement: Supplementary file 1 [file 99_Appendix_Surface.tex]

\section{CbV and CbN $\lam$-calculi: basic properties and surface factorization}
%Here and then everywhere in the appendix, we fix surface reduction to be as follows. 
%\begin{itemize}
%	\item CbN ($\betab=\beta$): $\surf =\head$   (the contextual closure of $\hh$).
%	\item CbV ($\betab=\betav$): $\surf= \weak$   (the contextual closure of $\ww$).
%\end{itemize}

\subsection{Contextual closure.}
In the proofs, we  exploit  some basic properties of the  contextual closure, which we collect here.
If a step $ T \redc T'$ is obtained by closure under \emph{non-empty context} of a rule $\rredc$, then  $T$ and $T'$ have \emph{the same shape, that is   both terms are an 
	application (resp. an abstraction, a variable, a term of shape $\opp{\dots}$).}
\begin{fact}[Shape preservation]\label{fact:shape} 
	Assume $T=\cc\hole{R}\red \cc\hole {R'}=T'$ and that the  context   $\cc$ is \emph{non-empty}. Then $T$ and $T'$ have the same shape.
	
	Hence,  for any non-surface step  $M \nsred M'$ ($\surf\in \{\head,\weak\}$) $M$ and $M'$ have the same shape.
\end{fact}

The following is an easy to verify consequence. %(see  Result \ref{sec:preservation} for details)
\begin{lemma}[Redexes preservation]\label{cor:redex} \hfill.
	\begin{enumerate}
		\item CbV. %Let $\red =\redbv \cup \redx{\op}$ and 
		%	Let $\surf\in \{\weak, \lsym,\RED{\rsym}\}$. 
		Assume  $T\nwredbv S$.  
		$T$ is a $\betav$-redex  \iff so is $S$.\\
		$T$ has shape $\opp{\dots}$ iff $S$ does.  
		\item CbN:  Assume  $T\nhredb S$.  
		$T$ is a $\beta$-redex \iff  so is $S$. \\
		$T$ has shape $\opp{\dots}$ iff $S$ does.  
	\end{enumerate}
\end{lemma}

\begin{lemma}[Surface normal forms]\label{lem:ex_nf}\label{lem:snf} Fixed a set of redexes $\R$, 
	$M$ is $\weak$-normal (resp. $\head$-normal) if there is no redex $R\in \R$ such that 	$M=\ww\hole R$ (resp. $M=\hh\hole R$)
	\begin{enumerate}
		\item \CbV. Let $\R$ be the set of $\betav$-redexes.
		Assume 
		$M \nwredbv M'$.
		%	{$M$ contains no $\weak$-redex  $\Leftrightarrow$ $M'$ contains no  $\weak$-redex.}	
		$M$ is   $\weak$-normal  $\Leftrightarrow$ $M'$ is     $\weak$-normal.
		
		\item \CbN. Let $\R$ be the set of $\betav$-redexes.	Assume $M \nhredb M'$.	
		%{$M$ contains no $\head$-redex  $\Leftrightarrow$ $M'$ contains no  $\head$-redex.}
		$M$ is   $\head$-normal  $\Leftrightarrow$ $M'$ is     $\head$-normal.
		
		\item Point 1. and 2. both  hold also taking for  $\R$ all the  terms of shape  $\opp{\dots M_i \dots}$
	\end{enumerate}
\end{lemma}
\begin{proof}By  induction on the shape of $M$.  Note that $M$ and ${M'}$ have the same shape, by \Cref{fact:shape}.
	\begin{enumerate}
		\item  $M\nwredbv M'$. We examine the shape of $M$.
		
		\begin{itemize}
			\item   $M\in \Val$ (and so ${M'}\in \Val$). The claim is trivial, because $M$ and $M'$ are $\weak$-normal.
			
			\item  $M=PQ$ and ${M'}=P'Q'$.  Either $P\nwred P'$ (and $Q'=Q$) or $Q\nwred Q'$ (and $P=P'$). 
			By using 	 the \ih, and \Cref{cor:redex}:
			
			(1) $M=PQ$ contains no $\weak$-redex\\ 
			$\Leftrightarrow$ ($P$ and $Q$ contain no $\weak$-redex, and $PQ$ is not a redex)  $\Leftrightarrow$\\ 
			$\Leftrightarrow$ ($P'$ and $Q'$ contain no $\weak$-redex, and $P'Q'$ is not a redex) $\Leftrightarrow$ \\ 
			(2)  $M'=P'Q'$ contains no $\weak$-redex

			%		\item $M=PQ$ and $N=P'Q'$.  Either $P\nsred P'$ (and $Q'=Q$) or $Q\nsred Q'$ (and $P=P'$). Assume $M=PQ$ is $\surf$-normal. Since $P$ and $Q$ are $\surf$-normal, by  \ih so are  $P'$ and $Q'$. Moreover, $N$ is not a redex, by Result \ref{cor:redex}, so $N$ is normal. Assuming $N=P'Q'$ normal is similar.
			\item $M=\opp{\dots M_i \dots}$ (and so $M'$ has the same shape).  The claim is trivial.
		\end{itemize}

		\item $M\nhredb M'$. Similar.
		
		\item  The proof is exactly the same, using again \Cref{cor:redex}.
	\end{enumerate}
\end{proof}

\subsection{Surface  Factorizations in CbV and CbN $\lam$-calculus}
We recall that every $\redb$-reduction sequence can be re-organized/factorized
as to first  performing head steps, and then everything else.  Similarly for $\redbv$-sequences and weak steps.
\begin{theorem}[Surface Factorizations]\label{thm:surf_factorization} \hfill

	\begin{itemize}
		\item  In $(\LambdaOp, \redb)$: 
		\begin{equation*}\tag{\emph{Head  Factorization}}
			\redb^* \ \subseteq \ \hredb^*  \cdot \nhredb^* 
		\end{equation*}

		\item In $(\LambdaOp, \redbv)$: 
		\begin{equation*}\tag{\emph{Weak  Factorization}}
			\redbv^* \ \subseteq \ \wredbv^*  \cdot \nwredbv^* 
		\end{equation*}

	\end{itemize}
\end{theorem}

\subsection{Probabilistic $\lam$-calculi: Surface Factorization and the need for \NDE}\label{sec:surface_factorization}
\label{app:proba}
%
%

%\paragraph{Surface Factorization} 
%\paragraph{CbN and CbV surface factorization}
$\PLambda^\cbn$  and  $\PLambda^\cbv$  each satisfies a  surface factorization (called finitary surface  standardization in \cite{FaggianRonchi}),  
taking into account the respective definition of surface reduction $\sred$ (weak reduction in CbV, head reduction in CbN):
\begin{equation*}\tag{Surface Factorization of $\Red$}
	\m \Red^*\n ~\timplies~ \m \sRed^*\cdot \nsRed^* \n
\end{equation*}

\paragraph{The need for \NDE.}
It is worth pointing out  the key role played here by the fact to adopt a $\NDS$-variant.
For both CbN and CbV, it is impossible to reorganize a $\Red$-sequence in such a way that the redexes are reduced from left to right.
\paragraph{CbN.}
The following is a counterexample (first noted in \cite{Alberti14}) to factorization via the usual deterministic head reduction. It is (a fortiori) also  a counter-example to leftmot-outermost factorization and to  left-to-right Standardization.
\begin{example}[CbN: leftmost factorization failure  \cite{Alberti14,LeventisThesis,FaggianRonchi}]\label{ex:counter}
	Consider the following $\Red$-sequence 
	\begin{center}
		{\footnotesize 	$\mset{(\lam x. \underline{I (y\oplus z)}) I} \allowbreak\Red  \mset{ (\lam x. \underline{y\oplus z}) I} \Red \mset{\two  \underline{(\lam x. y) I}, {\two}(\lam x.  z) I}  
			\xRedx{\head}{} \mset{{\two}y, {\two}(\lam x.  z) I}$}
	\end{center}
	% where  at   each step we underline the  redex which is fired. 
	Only  the last step fires  the proper head redex.  If we perform the head redex first, we have  $\mset{(\lam x.I (y\oplus z)) I}\Red \mset{I(y\oplus z)}$, from which 
	$\mset{{\two}y, {\two}(\lam x.  z) I}$ cannot be reached. 
\end{example}
%The counterexample does not invalidate the non-deterministic variant: indeed, the sequence   is  already a sequence of surface steps.
The counterexample does not invalidate the non-deterministic variant of head reduction.

}%SLV

\paragraph{CbV.} The following is a counter-example to factorization (and so also to standardization) via Plotkin's left reduction
\begin{example}[CbV: leftmost factorization failure]\label{counterex:standard}Let us consider the following sequence 
{\footnotesize 	$\mset{(II)(\underline{(\lam x. P\oplus Q)I})}\xRedx{\neg\lsym~}{} \mset{(II)(\underline{P\oplus Q} )} \xRedx{\neg\lsym~}{} \mset{\two (II)P, \two \underline{(II)}Q} \xRedx{\lsym~}{} \mset{\two IP,\two (II)Q}$}. 
Only the last step fires a left redex. If we perform the leftmost redex first, we have $\mset{(\underline{II})({(\lam x. P\oplus Q)I})}\xRedx{\lsym~}{}  \mset{I ((\lam x.P\oplus Q)I)}$, from 
where  $\mset{\two IP,\two (II)Q}$ cannot be reached. 
\end{example}		
Note that the counter-example does not invalidate  weak reduction in arbitrary order: indeed, the sequence   is  already a sequence of weak   steps.

\medskip
\SLV{}{\paragraph{The need to constrain probabilistic reduction (Confluence failure).}

\begin{example}[Failure of commutations]\label{ex:confluence_failure}	The key issue in calculi with choice  effects, as first   observed in \cite{deLiguoroP95} and well-discussed in \cite{LagoZ12}, resumes to 
	the difference between duplicating a coin (and then flipping it),  versus flipping a coin and duplicate the result. 
	The need for constraints on the probabilistic operator is exemplified by the 
	following well-known  counter-example to confluence \cite{deLiguoroP95, LagoZ12}, which  is a counter-example also to left-to-right standardization in its simpler form, head factorization. 
	In a CbN setting, 
	consider the duplicator $\Delta$, an effectful term  $ P = (I\oplus \Delta\Delta) $, and the following  two sequences from $\Delta P$:
	
	{\small \begin{itemize}
			\item $\mset{\Delta P }\nhred \mset{\two \Delta I, \two \Delta (\Delta\Delta)} \hred \mset{ \two II, \two (\Delta\Delta)(\Delta\Delta)}=\m$
			\item  $\mset{\Delta P} \hred   \mset{PP}=\m' $
	\end{itemize}}	
	
	\emph{Confluence failure}: $\m$ and $\m'$ have no common reduct.
	
	\emph{Head factorization failure}: from $\Delta P$ it is not possible to reach $\m$ performing head steps first.
\end{example}
}

%{\paragraph{The need to constrain probabilistic reduction (Confluence failure).}
%	
%	\begin{example}[Failure of commutations]	
	%		The need for constraints on the probabilistic operator is exemplified by the 
	%		following well-known  counter-example to confluence, which  is a counter-example also to left-to-right standardization in its simpler form, head factorization.
	%		In a CbN setting, 
	%		consider the duplicator $\Delta$, an effectful term  $ P = (I\oplus \Delta\Delta) $, and the following  two sequences from $\Delta P$:
	%		
	%		{\small \begin{itemize}
			%				\item $\mset{\Delta P }\nhred \mset{\two \Delta I, \two \Delta (\Delta\Delta)} \hred \mset{ \two II, \two (\Delta\Delta)(\Delta\Delta)}=\m$
			%				\item  $\mset{\Delta P} \hred   \mset{PP}=\m' $
			%		\end{itemize}}	
	%	
	%		\emph{Confluence failure}: $\m$ and $\m'$ have no common reduct.
	%		
	%		\emph{Head factorization failure}: from $\Delta P$ it is not possible to reach $\m$ performing head steps first.
	%	\end{example}
%}
